# Supplementary material for: Finite-Sample Convergence Bounds for Trust Region Policy Optimization in Mean-Field Games
Source: arXiv:2505.22781 source file (2025-05-28)
Supplement: Supplementary file 1 [file performance-difference.tex]

\begin{lemma}[Performance-difference lemma for different environments adapted from Lemma 3 of~\citealt{russo2019worst}]\label{lem:performance-difference-russo}
    Let us consider a MF-MDP $\cM = (\S, \A, \gamma, \rewardMDP, \kerMDP)$. Let $\pdist$ and $\pdist^\prime$ two population distributions. Consider a Markov chain generated by the rule $a_t \sim \policy(\cdot |s_t)$, $s_{t+1} \sim \kerMDP(\cdot|s_t,a_t, \pdist^\prime)$. Then it holds
    \begin{align}
        \JMFG(\policy, \pdist^\prime,s) - \JMFG(\policy, \pdist,s) &= \PE\left[ \sum_{t=0}^{\infty} \gamma^t \left(\rewardMDP(s_t,a_t, \pdist^\prime ) - \rewardMDP(s_t,a_t, \pdist)\right)\right] \\
        &+\PE\left[  \sum_{t=0}^{\infty} \gamma^t \left(\kerMDP \JMFG(\policy, \pdist,\cdot)(s_t, a_t, \pdist^\prime)    - \kerMDP \JMFG(\policy, \pdist,\cdot) (s_t, a_t, \pdist) \right)  \right] \eqsp.
    \end{align}
\end{lemma}
\begin{proof}
Using Bellman's equations, we have
\begin{align*}
\JMFG&(\policy, \pdist^\prime,s) - \JMFG(\policy, \pdist,s)  = \PE\left[ \rewardMDP(s_0,a_0, \pdist^\prime ) - \rewardMDP(s_0,a_0, \pdist)\right] \\
&+\PE\left[ \gamma \left(\kerMDP \JMFG(\policy, \pdist^\prime,\cdot)(s_0, a_0, \pdist^\prime)  - \kerMDP \JMFG(\policy, \pdist,\cdot) (s_0, a_0, \pdist)\right)   \right] \\
&= \PE\left[ \rewardMDP(s_0,a_0, \pdist^\prime ) - \rewardMDP(s_0,a_0, \pdist)\right] +\PE\left[ \gamma \left(\kerMDP \JMFG(\policy, \pdist,\cdot)(s_0, a_0, \pdist)  - \kerMDP \JMFG(\policy, \pdist,\cdot) (s_0, a_0, \pdist^\prime)\right)   \right] \\
&+\PE\left[ \gamma \left(\kerMDP (\JMFG(\policy, \pdist^\prime,\cdot) -  \JMFG(\policy, \pdist,\cdot)) (s_0, a_0, \pdist^\prime)\right)   \right] \\
&= \PE\left[ \rewardMDP(s_0,a_0, \pdist^\prime ) - \rewardMDP(s_0,a_0, \pdist)\right] +\PE\left[ \gamma \left(\kerMDP \JMFG(\policy, \pdist,\cdot)(s_0, a_0, \pdist)  - \kerMDP \JMFG(\policy, \pdist,\cdot) (s_0, a_0, \pdist^\prime)\right)   \right] \\
&+\gamma \PE\left[ (\JMFG(\policy, \pdist^\prime,s_1) -  \JMFG(\policy, \pdist,s_1))  \right] \eqsp.
\end{align*}
Unrolling the recursion yields the desired result.
\end{proof}

\begin{lemma}[Performance-difference lemma for different policies adapted from~\citet{mei2020global}]
\label{lem:performance_difference_lemma_mei}
We have
\begin{align*}
\valuefunc[][\theta^\prime, \pdist](\initdist) - \valuefunc[][\theta, \pdist](\initdist) = \frac{1}{1- \gamma} \sum_{s \in \S} d_{\initdist}^{\theta, \pdist}(s) \sum_{a \in \A}(\policy_{\theta^\prime}(a|s) -\policy_{\theta}(a|s)) \cdot \qfunc[][\theta^\prime, \pdist](s,a) \eqsp.
\end{align*}
\end{lemma}

\begin{lemma}
\label{lem:Lipschitz_stationnary}
Under assumption \Cref{assum:Lipschitz_reward_probability}, we have
\begin{align}
\Vert d^{\theta, \pdist} -  d^{\theta, \pdist^\prime} \Vert_1 \leq \nstates  L_{\pdist}^{\kerMDP}(\frac{\log_{\rho}(m^{-1})}{\log(\rho)} + (1- \rho)^{-1}) \Vert \pdist- \pdist^\prime \Vert_{1} \eqsp.
\end{align}
\end{lemma}
\begin{proof}
Following from Theorem 3.1 of~\citet{mitrophanov2005sensitivity}, we have
\begin{align}
\Vert d^{\theta, \pdist} -  d^{\theta, \pdist^\prime} \Vert_{TV} \leq  (\frac{\log_{\rho}(m^{-1})}{\log(\rho)} + (1- \rho)^{-1}) \Vert \kerMDP[\pdist][\theta]- \kerMDP[\pdist^\prime][\theta] \Vert_{\sup}\eqsp,
\end{align}
where $ \Vert \cdot \Vert_{\sup}$ is the operator norm: $\Vert K \Vert_{\sup} = \sup_{q}\Vert qK\Vert_{TV} = \sup_{q}\frac{1}{2}\Vert qK\Vert_{1}$. Applying \Cref{assum:Lipschitz_reward_probability}, we get
\begin{align}
\Vert d^{\theta, \pdist} -  d^{\theta, \pdist^\prime} \Vert_{1} \leq  \nstates  L_{\pdist}^{\kerMDP}(\frac{\log_{\rho}(m^{-1})}{\log(\rho)} + (1- \rho)^{-1}) \Vert \pdist- \pdist^\prime \Vert_{1}\eqsp,
\end{align}
\end{proof}

\begin{lemma}[Ascent lemma for smooth functions]
\label{lem:ascent_lemma}
Let $f:\rset^d \rightarrow \rset$ be a $\beta$-smooth function, $\theta \in \rset^d$ and $\theta^\prime = \theta + \frac{1}{\beta} \frac{\partial f}{\partial \theta}$ then we have
\begin{align*}
f(\theta) - f(\theta^\prime) \leq \frac{-1}{2 \beta} \cdot \left\Vert \frac{\partial f(\theta)}{\partial \theta} \right\Vert_2^2 \eqsp.
\end{align*}
\end{lemma}

\begin{lemma}[Lemma C.1 of~\citet{agarwal2020optimality}]
The gradient of the value function w.r.t $\theta(s,a)$ is equal to
\begin{align*}
\frac{\partial \valuefunc[][\theta, \pdist](\initdist)}{\partial \theta(s,a)} = \frac{1}{1- \gamma} d_{\initdist}^{\theta, \pdist}(s)\policy_{\theta}(a|s) A^{\theta , \pdist}(s,a) \eqsp,
\end{align*}
where $A^{\theta , \pdist}$ is the advantage function defined as $A^{\theta , \pdist}(s,a) = \qfunc[][\theta, \pdist](s,a) - \valuefunc[][\theta, \pdist](s)$.
\end{lemma}

\begin{lemma}[Lipschitz property of multiplication]
\label{lem:lipshitz_multiplication}
Suppose $f(x)$ and $g(x)$ are two functions bounded by $C_f$ and $C_g$, and are $L_f$- and $L_g$-Lipschitz continuous, then $f(x)g(x)$ is $(C_f L_g + C_g L_f)$-Lipschitz continuous.
\end{lemma}

\begin{proof}
\begin{align*}
\|f(x_1)g(x_1) - f(x_2)g(x_2)\| 
&= \|f(x_1)g(x_1) - f(x_1)g(x_2) + f(x_1)g(x_2) - f(x_2)g(x_2)\| \\
&\leq \|f(x_1)\|\|g(x_1) - g(x_2)\| + \|f(x_1) - f(x_2)\|\|g(x_2)\| \\
&\leq (C_f L_g + C_g L_f)\|x_1 - x_2\|.
\end{align*}
\end{proof}
